# Supplementary material for: Observation of the decays $B_{(s)}^{0}\to D_{s1}(2536)^{\mp}K^{\pm}$
Source: arXiv:2308.00587 source file (2023-10-24)
Supplement: Supplementary file 1 [file appendix.tex]

\appendix

\section{Angular decay rate}\label{sec:app:angular_decay_rate}

\subsection{Helicity-based matrix element}
\label{sec:ang:tot_matix_element}
According to Ref. \cite{Richman:1984gh}, the matrix element for a two-body decay, $A\rightarrow B+C$, can be written as 
\begin{gather}
    \mathcal{M}_{A\rightarrow BC} = \mathcal{H}^{A\rightarrow BC}_{\lambda_B, \lambda_C}\mathcal{D}^{J_A}_{m_A, \lambda_B-\lambda_C}(\phi_B,\theta_B,-\phi_B)^{*},
\end{gather}
where $\mathcal{H}^{A\rightarrow BC}_{\lambda_B, \lambda_C}$ is the helicity coupling featuring the strength of the helicity-base partial wave, and $\mathcal{D}^{J_A}_{m_A, \lambda_B-\lambda_C}(\phi_B,\theta_B,-\phi_B)^{*}$ determines the corresponding angular property. Here the helicity coupling $\mathcal{H}^{A\rightarrow BC}_{\lambda_B, \lambda_C}$ is a complex number. 
If the $A\rightarrow BC$ decay is a strong or electromagnetic process, the parity conservation requires that 
\begin{gather}
    \mathcal{H}^{A\rightarrow BC}_{-\lambda_B, -\lambda_C} = P_A P_B P_C (-1)^{J_B+J_C-J_A}\mathcal{H}^{A\rightarrow BC}_{\lambda_B, \lambda_C},
\end{gather}
where $P$ indicates the intrinsic parity of corresponding particle, and this relation can be used to reduce the number of parameters in the total decay amplitude. An alternative way to characterise the relative strength of the partial waves is to use $LS$ representation, where $L$ stands for the orbital angular momentum between the two decay products and $S$ is the total spin of them. The helicity coupling $\mathcal{H}^{A\rightarrow BC}_{\lambda_B, \lambda_C}$ and the $LS$ coupling $B_{LS}$ are associated by 
\begin{align}
\mathcal{H}^{A\rightarrow BC}_{\lambda_B, \lambda_C} =& \sum_{L,S}\sqrt{\frac{2L+1}{2J_A+1}}B_{LS}\times \braket{J_A,J_B,\lambda_A,\lambda_B}{S, \lambda_B-\lambda_C}\\\notag
&\times \braket{L,S,0,\lambda_B-\lambda_C}{J_A, \lambda_B-\lambda_C}.
\end{align}
If the mass of particle $A$ is close to the threshold of the $BC$ system, namely $\frac{m_A}{m_B+m_C}\approx 1$, the magnitude of $B_{LS}$ with higher $L$ value are usually suppressed due to the angular momentum barrier effect.

The angular dependence of the two-body decay amplitude is described by the Wigner-D function, which is defined as
\begin{gather}
    \mathcal{D}^{J}_{m,m^\prime}(\alpha, \beta, \gamma) = \bra{J,m} R_z(\alpha)R_y(\beta)R_z(\gamma)\ket{J,m^\prime} = e^{-im\alpha}d^{J}_{m,m^\prime}(\beta)e^{-im^\prime \gamma},
\end{gather}
where $R_z$ ($R_y$) indicates the rotation operator along the $z$  ($y$) axis. 
The angular variables $\phi_B$ and $\theta_B$ correspond to the azimuthal and polar angles of $\vec{p}^A_B$, namely the direction of particle $B$'s momentum in the ($x_0^A, y_0^A, z_0^A$) coordinate system, \ie 
\begin{gather}
    \phi_B = \tan^{-1}\left(\frac{\vec{y}_0^A \cdot \vec{p}^A_B}{\vec{x}_0^A \cdot \vec{p}^A_B}\right)\quad\text{and}\quad  
    \theta_B = \cos^{-1}\left( \frac{\vec{z}_0^A \cdot \vec{p}^A_B}{|\vec{p}^A_B|}\right),
\end{gather}
where $\tan^{-1}(y/x)$ is the principal value of the arctangent of $y/x$, which takes into account the quadrant where the point ($x$, $y$) locates.

The total matrix element for the \BdsDsoK signal channels is obtained by a product of matrix elements of all the two-body decays involved. Taking the \BsDsoK decay for example,  it is written by
\begin{align}
    \mathcal{M}^{\tot} =& \sum_{\lambda_{\Dstarzb}} \mathcal{H}^{\decay{\Bs}{\Dsom\Kp}}_{\lambda_\Dsom,\lambda_\Kp} \mathcal{H}^{\decay{\Dsom}{\Dstarzb\Km}}_{\lambda_\Dstarzb,\lambda_\Km} \mathcal{H}^{\decay{\Dstarzb}{\Dzb\gamma(\piz)}}_{\lambda_\Dzb,\lambda_{\gamma(\piz)}}\\ \notag
    &\times D^{J_{\Bs}}_{m_{\Bs},\lambda_{\Dsom}-\lambda_{\Kp}}(\phi_{\D_{s1}},\theta_{\D_{s1}},-\phi_{\D_{s1}})^{*} \\\notag
    &\times D^{J_{\Dsom}}_{m_{\Dsom}, \lambda_{\Dstarzb}-\lambda_{\Km}}(\phi_{\Dstar},\theta_{\Dstar},-\phi_{\Dstar})^* \\\notag
    &\times D^{J_{\Dstarzb}}_{m_{\Dstarzb}, \lambda_{\Dzb}-\lambda_{\gamma(\piz)}}(\phi_{\D}, \theta_{\D}, -\phi_{\D})^* .\notag
\end{align}
The particle's helicity is defined in the \Bs rest frame for \Dsom and \Kp mesons, in the \Dsom rest frame for \Dstarzb and \Km mesons, and in the \Dstarzb rest frame for \Dzb meson and the $\gamma$ or \piz meson.
For the \decay{\Bs}{\Dsomp\Kpm} two-body decay, the direction of three axes can be arbitrarily defined. We define that the $z$ axis is the direction of the momentum of $\Dsom$ meson and the $x$ axis is in the \Dsom decay plane.
With this definition, $\mathcal{M}^{\tot}$ is simplified as 
    \begin{align}
        \mathcal{M}^{tot} =& \sum_{\lambda_{\Dstarzb}} \mathcal{H}^{\decay{\Bs}{\Dsom\Kp}}_{\lambda_\Dsom,\lambda_\Kp} \mathcal{H}^{\decay{\Dsom}{\Dstarzb\Km}}_{\lambda_\Dstarzb,\lambda_\Km} \mathcal{H}^{\decay{\Dstarzb}{\Dzb\gamma(\piz)}}_{\lambda_\Dzb,\lambda_{\gamma(\piz)}}\\ \notag
        % &\times D^{}_{0,0}(0,0,0)^{*} D^{1}_{0, \lambda_{\Dstarzb}}(0,\theta^{\prime},0)^* D^{1}_{\lambda_{\Dstarzb}, -\lambda_{\gamma(\piz)}}(\phi_{\Dzb}, \theta_{\Dzb}, -\phi_{\Dzb})^*
        &\times D^{J_{\Bs}}_{m_{\Bs},\lambda_{\Dsom}-\lambda_{\Kp}}(0, 0, 0)^{*} \times D^{J_{\Dsom}}_{m_{\Dsom}, \lambda_{\Dstarzb}-\lambda_{\Km}}(0,\theta_{\Dstar},0)^* \\\notag
        &\times D^{J_{\Dstarzb}}_{m_{\Dstarzb}, \lambda_{\Dzb}-\lambda_{\gamma(\piz)}}(\chi, \theta_{\D}, -\chi)^* .\notag
    \end{align}

\begin{table}[!t]
    \centering
    \caption{
    Spin-parity numbers and helicities for particles involved in the signal decay chain.}
    \label{tab:angular:JP_number}
    \begin{tabular}{c | c c c c c c c}
        \toprule[1pt]
        &\Bs & \Dsom & $\Dstarzb$ & \Dzb & \Kpm & $\gamma$ & \piz \\
        \midrule[0.5pt]
        $J^P$ & $0^-$ & $1^+$ & $1^-$ & $0^-$ & $0^-$ & $1^-$ & $0^-$\\
        helicity & 0 & 0 & $0,\pm1$ & 0 & 0 & $\pm1$ & 0\\
        \bottomrule[1pt]
    \end{tabular}
\end{table}
For the series decays in the \decay{\Bs}{\Dsomp\Kpm} channel, the spin-parity numbers $J^P$ of all the particles involved are listed in Table~\ref{tab:angular:JP_number}. 
The helicities of these particles according to the conservation of angular momentum are also listed in this table. 
Here the helicity of $\Dstarzb$ meson $\lambda_{\Dstarzb}$ is undetermined in the $\decay{\Dsom}{\Dstarzb\Km}$ sub-decay process, so the total decay amplitude $\mathcal{M}^{\tot}$ needs to sum over $\lambda_{\Dstarzb}$. 
Substituting the determined helicity of the particles into $\mathcal{M}^{\tot}$, we can further simplify it as
    \begin{align}
        \mathcal{M}^{tot} =& \sum_{\lambda_{\Dstarzb}} \mathcal{H}^{\decay{\Bs}{\Dsom\Kp}}_{0,0} \mathcal{H}^{\decay{\Dsom}{\Dstarzb\Km}}_{\lambda_\Dstarzb,0} \mathcal{H}^{\decay{\Dstarzb}{\Dzb\gamma(\piz)}}_{0,\lambda_{\gamma(\piz)}}\\ \notag
        &\times D^{}_{0,0}(0,0,0)^{*} D^{1}_{0, \lambda_{\Dstarzb}}(0,\theta_{\Dstar},0)^* D^{1}_{\lambda_{\Dstarzb}, -\lambda_{\gamma(\piz)}}(\chi, \theta_{\D}, -\chi)^* .
    \end{align}
To simplify the notation, $\mathcal{H}^{\decay{\Bs}{\Dsom\Kp}}_{0,0} \mathcal{H}^{\decay{\Dsom}{\Dstarzb\Km}}_{\lambda_\Dstarzb,0} \mathcal{H}^{\decay{\Dstarzb}{\Dzb\gamma}}_{0,\lambda_{\gamma}}$, is denoted as $A_{\lambda_{\Dstarzb},\lambda_{\gamma}}$ below, and  $\mathcal{H}^{\decay{\Bs}{\Dsom\Kp}}_{0,0} \mathcal{H}^{\decay{\Dsom}{\Dstarzb\Km}}_{\lambda_\Dstarzb,0} \mathcal{H}^{\decay{\Dstarzb}{\Dzb\piz}}_{0,\lambda_{\piz}}$ as $B_{\lambda_{\Dstarzb},\lambda_{\piz}}$.
%for clean notations.

The full matrix element squared, also named as the angular distribution, used in the photon chain is written as 
\begin{gather}
    |\mathcal{M}|^{2} = \sum_{\lambda_{\gamma} = \pm1} \left|\sum_{\lambda_{\Dstarzb}=0,\pm1} A_{\lambda_{\Dstarzb},\lambda_{\gamma}}\times D^{}_{0,0}(0,0,0)^{*} D^{1}_{0, \lambda_{\Dstar}}(0,\theta_{\Dstar},0)^* D^{1}_{\lambda_{\Dstarzb}, -\lambda_{\gamma}}(\chi, \theta_{\D}, -\chi)^* \right|^2 .\label{equ:app:angular:Msq_gamma_before}
\end{gather}
For the $\piz$ chain, it is written as 
\begin{gather}
    |\mathcal{M}|^{2} = \sum_{\lambda_{\piz}=0} \left| \sum_{\lambda_\Dstarzb = 0,\pm1}B_{\lambda_{\Dstarzb},\lambda_{\piz}}\times D^{}_{0,0}(0,0,0)^{*} D^{1}_{0, \lambda_{\Dstarzb}}(0,\theta_{\Dstar},0)^* D^{1}_{\lambda_{\Dstarzb}, -\lambda_{\piz}}(\chi, \theta_{\D}, -\chi)^* \right|^2 .\label{equ:app:angular:Msq_piz_before}
\end{gather}
Due to the parity conservation, $A_{\lambda_\Dstarzb, 1}=-A_{\lambda_\Dstarzb, -1}$, $A_{-1,\lambda_\gamma}=A_{1,\lambda_\gamma}$, and $B_{-1, \lambda_\piz}=B_{1, \lambda_\piz}$. 
Below we label $A_{0,1}$ as $A_{0}$, $A_{1,1}$ as $A_{1}$, $B_{0,0}$ as $B_{0}$, and $B_{1,0}$ as $B_{1}$, to simplify the notation.

Taking the formula of Wigner-D function into Eq.~\ref{equ:app:angular:Msq_gamma_before} and \ref{equ:app:angular:Msq_piz_before}, the differential decay rate can be reduced to 
    \begin{align}\label{equ:app:angular:Msq_gamma_reduction}
    \frac{\deriv^3 \Gamma}{\deriv \cos \theta_{\Dstar} \deriv \cos \theta_{\D} \deriv \chi} \propto & \cos^2\theta_{\Dstar}\sin^2\theta_{\D} A_0^2 + \sin^2\theta_\Dstar (\sin^2\chi + \cos^2\chi \cos^2\theta_D)k^2A_0^2\\\notag
        &+ 2\cos\chi\sin\theta_{\Dstar}\cos\theta_{\Dstar}\sin\theta_{\D}\cos\theta_{\D} k\cos\phi A_0^2 
    \end{align}
for photon decay chain;
    \begin{align}\label{equ:app:angular:Msq_piz_reduction}
    \frac{\deriv^3 \Gamma}{\deriv \cos \theta_{\Dstar} \deriv \cos \theta_{\D} \deriv \chi} \propto & \cos^2\theta_{\Dstar}\cos^2\theta_{\D}B_0^2+\cos^2\chi\sin^2\theta_{\Dstar}\sin^2\theta_{\D}k^2B_0^2 \\ \notag
        & - 2\cos\chi\sin\theta_{\Dstar}\cos\theta_{\Dstar}\sin\theta_{\D}\cos\theta_{\D}k\cos\phi B_0^2 
    \end{align}
for $\piz$ chain, where we defined $A_1(B_1) = ke^{i\phi}A_0 (B_0)$ with $k>0$ and $\phi \in(-\pi, \pi]$. The details of simplification can be found in the following Appendix \ref{sec:appendix:cal_decay}.

\subsection{The detail of calculating procedure}\label{sec:appendix:cal_decay}
We have given the simplified Eqs.~\ref{equ:app:angular:Msq_gamma_before} and \ref{equ:app:angular:Msq_piz_before} in Appendix~\ref{sec:ang:tot_matix_element}. Taking the photon chain as example, this expression can be reduced to 

    \begin{equation}
        \label{equ:appendix:cal_decay:first}
    \begin{split}
        &\frac{\deriv^3 \Gamma}{\deriv \cos \theta_{\Dstar} \deriv \cos \theta_{\D} \deriv \chi} \propto|\mathcal{M}|^2 \\
        &= \sum_{\lambda_{\gamma} =\pm1}\left|\sum_{\lambda_{\Dstarzb}=0,\pm1}\left[ A_{\lambda_{\Dstarzb}, \lambda_{\gamma}}D^{0}_{0,0}(0,0,0)^{*} D^{1}_{0,\lambda_{\Dstarzb}}(0,\theta_{\Dstar},0)^{*} D^{1}_{\lambda_{\Dstarzb},-\lambda_\gamma}(\chi,\theta_{\D},-\chi)^{*}\right]\right|^2 \\
        &= \left|\sum_{\lambda_{\Dstarzb}=0,\pm1}\left[ A_{\lambda_{\Dstarzb},1} D^{0}_{0,0}(0, 0, 0)^{*}D^{1}_{0,\lambda_{\Dstarzb}}(0,\theta_{\Dstar},0)^{*} D^{1}_{\lambda_{\Dstarzb},-1}(\chi,\theta_{\D},-\chi)^{*}\right]\right|^2 \\
        &+\left|\sum_{\lambda_{\Dstarzb}=0,\pm1}\left[A_{\lambda_{\Dstarzb},-1} D^{0}_{0,0}(0,0,0)^{*} D^{1}_{0,\lambda_{\Dstarz}}(0,\theta_{\Dstar},0)^{*} D^{1}_{\lambda_{\Dstarz},1}(\chi,\theta_{\D},-\chi)^{*} \right]\right|^2 \\
        &= \left|(D^{0*}_{0,0})^1(D^{1*}_{0,0})^2(D^{1*}_{0,-1})^3 A_{0,1}+(D^{0*}_{0,0})^1(D^{1*}_{0,1})^2(D^{1*}_{1,-1})^3 A_{1,1}\right. \\
        &+\left.(D^{0*}_{0,0})^1(D^{1*}_{0,-1})^2(D^{1*}_{-1,-1})^3 A_{-1, 1}\right|^2+\left|(D^{0*}_{0,0})^1(D^{1*}_{0,0})^2(D^{1*}_{0,1})^3 A_{0,-1}\right. \\
        &+\left.(D^{0*}_{0,0})^1(D^{1*}_{0,1})^2(D^{1*}_{1,1})^3 A_{1,-1}+(D^{0*}_{0,0})^1(D^{1*}_{0,-1})^2(D^{1*}_{-1,1})^3 A_{-1,-1}\right|^2,
    \end{split}
    \end{equation}
where $(D^j_{m,m^\prime})^1\equiv D^j_{m,m^\prime}(0,0,0)$, $(D^j_{m,m^\prime})^2\equiv D^j_{m,m^\prime}(0,\theta_{\Dstar},0)$ and $(D^j_{m,m^\prime})^3\equiv D^j_{m,m^\prime}(\chi,\theta_{\D},-\chi)$. Here $A_{\lambda_\Dstarzb, 1}$ is the negative of $A_{\lambda_\Dstarzb, -1}$ and $A_{-1,\lambda_\gamma}$ is equal to $A_{1,\lambda_\gamma}$ due to parity conservation. We label $A_{0,1}$ as $A_{0}$ and $A_{1,1}$ as $A_{1}$. In the remaining part of this note, we take these notations for clarity. Then the angular distribution can be further reduced to

    \begin{align}
    \frac{\deriv^3 \Gamma}{\deriv \cos \theta_{\Dstar} \deriv \cos \theta_{\D} \deriv \chi} \propto &\left|-\cos\theta_{\Dstar} \frac{\sqrt{2}}{2}\sin\theta_{\D}e^{i\chi}A_0\right.\\\notag
    &\left.+\frac{\sqrt{2}}{2}\left(\sin\theta_{\Dstar}e^{i\chi} \frac{1-\cos\theta_{\D}}{2}e^{i\chi}-\sin\theta_{\Dstar}e^{i\chi}\frac{1+\cos\theta_{\D}}{2}e^{-i\chi}\right) A_1\right|^2\\\notag
    &+\left|\cos\theta_{\Dstar}\frac{\sqrt{2}}{2}\sin\theta_{\D}e^{-i\chi}A_0\right.\\\notag
    &\left.+\frac{\sqrt{2}}{2}\left(\sin\theta_{\Dstar}e^{-i\chi}\frac{1+\cos\theta_{\D}}{2}e^{i\chi}-\sin\theta_{\Dstar}e^{-i\chi}\frac{1-\cos\theta_{\D}}{2}e^{-i\chi}\right)A_1\right|^2.\\\notag
    & = \cos^2\theta_{\Dstar}\sin^2\theta_{\D}A_0 A_0^* + 
    \left( \sin^2\chi\sin^2\theta_{\Dstar}+ \cos^2\chi\sin^2\theta_{\Dstar}\cos^2\theta_{\D}\right) A_1 A_1^*\\\notag
    &+ 2\cos\chi\sin\theta_{\Dstar}\cos\theta_{\Dstar}\sin\theta_{\D}\cos\theta_{\D}(A_0 A_1^* + A_1 A_0^*)/2
    \end{align}
As the relation between $A_1$ and $A_0$ is $A_1 = ke^{i\phi}A_0$, the final expression is:
    \begin{align}
    \frac{\deriv^3 \Gamma}{\deriv \cos \theta_{\Dstar} \deriv \cos \theta_{\D} \deriv \chi} \propto &\cos^2\theta_{\Dstar}\sin^2\theta_{\D}A_0^2 +
    \left( \sin^2\phi\sin^2\theta_{\Dstar}+ \cos^2\chi\sin^2\theta_{\Dstar}\cos^2\theta_{\D}\right)k^2A_0^2\\\notag
    &+ 2\cos\chi\sin\theta_{\Dstar}\cos\theta_{\Dstar}\sin\theta_{\D}\cos\theta_{\D}k\cos\phi A_0^2.
    \end{align}

\clearpage
